# Supplementary material for: Chemotaxis of cargo-carrying self-propelled particles
Source: arXiv:2009.09060 ancillary file (2020-09-18)
Supplement: Supplementary file 1 [file sm.pdf]

# Suplemental Material: Chemotaxis of cargo-carrying self-propelled particles

Hidde D. Vuijk, Holger Merlitz, Michael Lang, Abhinav Sharma, Jens-Uwe Sommer

## I. OUTLINE

In these supplemental materials, details of the derivations are shown. All results hold for two and three dimensions and for both active Brownian particles (ABPs) and run-and-tumble particles (RTPs). Section II shows the derivation of the steady-state density of the active-passive dimer with a rigid bond in a swim force gradient (Eq. 1 in the main text), as well as the derivation for a dimer with a harmonic bond with zero rest length. Section II D shows the derivation of the Born-Oppenheimer approximation for the $q \to \infty$ limit (Eqs. 3 and 4 in the main text). Section II E shows the derivation of the average position of the dimer in a rectangular box as in Fig. 3 of the main text. In Section III we comment on how the model relates to a dimer with a passive Brownian particle in a temperature gradient in stead of an ABP with a swim-force gradient. In Section IV we show the derivation of the density for a dimer in one dimension and consider the effect of the spring constant of the potential between the active and passive particle on the steady-state density. Furthermore, we consider numerically a anharmonic potential to show that the transition to chemotaxis exist for a wide range of potentials, and briefly discuss a possible experimental setup to test the theory.

## II. COURSE GRAINING THE ACTIVE-PASSIVE DIMER

The derivations shown here rely on two coarse-graining steps. First, the orientational degrees of freedom are eliminated from the Fokker-Planck Equation (FPE) by expanding in eigenfunctions of the Laplacian on the unit sphere. This results in a hierarchy of equations for functions that depend only on the position coordinates of the active particle and the cargo particle. This method is based on the adiabatic elimination by the eigenfunction expansion method developed in ref. [1] and has been used to study both interacting and noninteracting active Brownian particles [2–6]. Second, because we are interested in the large-scale behaviour of the system (that is, length scales much larger that the separation between the two particles), we integrate out the internal degrees of freedom. Because of this second coarse-graining step, one does not need to determine explicitly the expansion coefficients in the expansion in eigenfunctions of the Laplacian, and the combination of the two steps results in accurate predictions for the relevant quantities.

### A. The active-passive dimer model

The equations of motion for an ABP [7] bound to a passive cargo particle are

$$\frac{\partial}{\partial t}\boldsymbol{r}_1 = \frac{1}{\gamma}\boldsymbol{F} + \frac{1}{\gamma}f_s(\boldsymbol{r}_1)\boldsymbol{p} + \sqrt{2T/\gamma}\boldsymbol{\xi}_1, \tag{1}$$

$$\frac{\partial}{\partial t}\boldsymbol{p} = \sqrt{2D_r}\boldsymbol{p}\times\boldsymbol{\eta} + \text{tumble}, \tag{2}$$

$$\frac{\partial}{\partial t}\boldsymbol{r}_2 = -\frac{1}{q\gamma}\boldsymbol{F} + \sqrt{2T/q\gamma}\boldsymbol{\xi}_2, \tag{3}$$

where $\boldsymbol{r}_1$ is the coordinate of the active particle and $\boldsymbol{r}_2$ the coordinate of the (passive) cargo particle, $\boldsymbol{p}$ is the orientation of the active particle, and $\boldsymbol{F}$ is the force the cargo particle exerts on the active particle. The orientation vector changes because of orientational diffusion and because of tumbling, which means that with rate $\alpha$ the orientation vector changes to a random position on the unit sphere. $T$ is the temperature in units such that the Boltzmann constant $k_b$ is unity. The friction of the active particle is $\gamma$. The friction of the passive cargo particle is $q$ times that of the active particle. The swim force of the active particle is $f_s$. (The swim speed is $v_s = f_s/\gamma$.) The vectors $\boldsymbol{\xi}_1$, $\boldsymbol{\xi}_2$ and $\boldsymbol{\eta}$ are random Gaussian vectors with zero mean and autocorrelation $\langle\boldsymbol{\xi}_1(t)\boldsymbol{\xi}_1(t')\rangle = \langle\boldsymbol{\xi}_2(t)\boldsymbol{\xi}_2(t')\rangle = \langle\boldsymbol{\eta}(t)\boldsymbol{\eta}(t')\rangle = \mathbf{1}\delta(t-t')$, where $\mathbf{1}$ is the identity matrix.

The potential holding the two particles together is

$$U(\boldsymbol{r}_1, \boldsymbol{r}_2) = \frac{1}{2}k(|\boldsymbol{r}_1 - \boldsymbol{r}_2| - l_0)^2, \tag{4}$$

where $k$ is the spring constant, and $l_0$ is the rest length. We consider two cases: i) A rigid bond, which we model by taking the limit $k \to \infty$. ii) A harmonic spring with zero rest length ($l_0 = 0$) and general spring constant k. The force on the active particle is $\boldsymbol{F} = -\nabla_1 U = -k(r' - l_0)\hat{\boldsymbol{r}}'$, where $\boldsymbol{r}' = \boldsymbol{r}_1 - \boldsymbol{r}_2$, $r' = |\boldsymbol{r}'|$, and $\hat{\boldsymbol{r}}' = \boldsymbol{r}'/r'$. The force on the passive particle is $-\boldsymbol{F}$. Other kinds of potentials are considered in Section IV.

The Fokker-Planck equation (FPE) corresponding Eqs. (1), (2) and (3) is [8]

$$\begin{aligned}\frac{\partial}{\partial t}P(t) = &-\frac{1}{\gamma}\nabla_1\cdot[\boldsymbol{F}P(t)] - \frac{1}{\gamma}\nabla_1\cdot[f_s\boldsymbol{p}P(t)]\\ &+\frac{T}{\gamma}\nabla_1^2P(t) + D_r\boldsymbol{\mathcal{R}}^2P(t)\\ &+\frac{1}{q\gamma}\nabla_2\cdot[\boldsymbol{F}P(t)] + \frac{T}{q\gamma}\nabla_2^2P(t)\\ &-\alpha P(t) + \alpha\phi(t),\end{aligned} \tag{5}$$

where $P(t) = P(\boldsymbol{r}_1, \boldsymbol{r}_2, \boldsymbol{p}, t)$ and $\boldsymbol{\mathcal{R}} = \boldsymbol{p} \times \nabla_{\boldsymbol{p}}$ is the angular momentum operator in the space of $\boldsymbol{p}$ [9], and $\boldsymbol{\mathcal{R}}^2$ is the Laplacian on the unit sphere. The last two terms account for tumbling with rate $\alpha$ [2]. And $\phi(t) = \phi(\boldsymbol{r}_1, \boldsymbol{r}_2, t) = \int d\Omega_d P(\boldsymbol{r}_1, \boldsymbol{r}_2, \boldsymbol{p}(\Omega_d), t)$, with $\Omega_d$ the d-dimensional solid angle ($\Omega_2 = 2\pi$, $\int d\Omega_2 = \int_0^{2\pi} d\theta \sin\theta$, $\Omega_3 = 4\pi$, $\int d\Omega_3 = \int_0^{\pi} d\phi \int_0^{2\pi} d\theta \sin\theta$).

### B. Eliminating the orientational degrees of freedom

To find an equation for the density, we expand $P(t)$ in eigenfunctions of the $\boldsymbol{\mathcal{R}}^2$ operator and integrate out the orientational degrees of freedom. The first three eigenfunctions of $\boldsymbol{\mathcal{R}}^2$ are 1, $\boldsymbol{p}$, $\boldsymbol{Q} = \boldsymbol{pp} - \boldsymbol{1}/d$. The eigenvalues are, respectively, 0, $-(d-1)$ and $-2d$. The probability can be expanded in the eigenfunctions of $\boldsymbol{\mathcal{R}}^2$ as [3, 4]

$$P(t) = \phi + \boldsymbol{\sigma} \cdot \boldsymbol{p} + \boldsymbol{\omega} : \boldsymbol{Q} + \Theta\left(P(t)\right), \tag{6}$$

where $\boldsymbol{Q} = \boldsymbol{pp} - \boldsymbol{1}/d$. This is the Cartesian multipole expansion. One could equivalently use a angular multipole expansion, where $P(t)$ is expanded in spherical harmonics (or circular harmonics for $d = 2$) [10]. The functions $\phi$, $\boldsymbol{\sigma}$ and $\boldsymbol{\omega}$ depend on $\boldsymbol{r}_1$, $\boldsymbol{r}_2$ and $t$. $\boldsymbol{\sigma}$ and $\boldsymbol{\omega}$ are the dipole and quadrupole moments, and are proportional to the polar and nematic order parameter [11]. Note that $\boldsymbol{\omega}$ can be made symmetric and traceless [4].

Next we define the scalar product

$$\langle f(\boldsymbol{p}), g(\boldsymbol{p}) \rangle = \int d\Omega_d f(\boldsymbol{p}(\Omega_d))\; g(\boldsymbol{p}(\Omega_d)). \tag{7}$$

Note that $\langle f(\boldsymbol{p}), g(\boldsymbol{p}) \rangle = \langle f(\boldsymbol{p}) g(\boldsymbol{p}), 1 \rangle$ and that with this scalar product $\boldsymbol{\mathcal{R}}^2$ is Hermitian: $\left\langle f(\boldsymbol{p}), \boldsymbol{\mathcal{R}}^2 g(\boldsymbol{p}) \right\rangle = \left\langle \boldsymbol{\mathcal{R}}^2 f(\boldsymbol{p}), g(\boldsymbol{p}) \right\rangle$. Furthermore, the following equations are used in the derivations [4]:

$$\langle p_i, p_j \rangle = \frac{\Omega_d}{d} \delta_{ij}, \tag{8}$$

$$\langle p_i p_j, p_k, p_l \rangle = \frac{\Omega_d}{d(d+2)} \left( \delta_{ik}\delta_{jl} + \delta_{il}\delta_{kj} + \delta_{ik}\delta_{jk} \right), \tag{9}$$

$$\begin{aligned} \langle Q_{ij}, Q_{kl} \rangle &= \frac{\Omega_d}{d} \frac{1}{2+d} \left( \delta_{ik}\delta_{jl} + \delta_{il}\delta_{jk} - \frac{2}{d} \delta_{ij}\delta_{kl} \right), \\ &\equiv \frac{\Omega_d}{d} \frac{2}{2+d} A_{ijkl}, \end{aligned} \tag{10}$$

and because 1, $\boldsymbol{p}$, and $\boldsymbol{Q}$ as well as the higher order moments are orthogonal

$$\langle 1, 1 \rangle = \Omega_d, \tag{11}$$

$$\langle \boldsymbol{p}, 1 \rangle = 0, \tag{12}$$

$$\langle \boldsymbol{Q}, 1 \rangle = 0, \tag{13}$$

$$\langle 1, P(t) \rangle = \phi \Omega_d, \tag{14}$$

$$\langle \boldsymbol{p}, P(t) \rangle = \sigma \cdot \langle \boldsymbol{p}, \boldsymbol{p} \rangle, \tag{15}$$

$$\langle \boldsymbol{Q}, P(t) \rangle = \boldsymbol{\omega} : \langle \boldsymbol{Q}, \boldsymbol{Q} \rangle, \tag{16}$$

$$\langle 1, \Theta(P(t)) \rangle = 0, \tag{17}$$

$$\langle \boldsymbol{p}, \Theta(P(t)) \rangle = 0, \tag{18}$$

$$\langle \boldsymbol{Q}, \Theta(P(t)) \rangle = 0. \tag{19}$$

Because most operators in Eq. (5) do not depend on $\boldsymbol{p}$, we rewrite it as

$$\begin{aligned} \frac{\partial}{\partial t} P(t) =& L P(t) + \boldsymbol{L}_s \cdot [\boldsymbol{p} P(t)] + D_r \boldsymbol{\mathcal{R}}^2 P(t) \\ & - \alpha P(t) + \alpha \phi, \end{aligned} \tag{20}$$

where

$$\begin{aligned} L P(t) =& -\frac{1}{\gamma} \nabla_1 \cdot [\boldsymbol{F} P(t)] + \frac{T}{\gamma} \nabla_1^2 P(t) \\ & + \frac{1}{q\gamma} \nabla_2 \cdot [\boldsymbol{F} P(t)] + \frac{T}{q\gamma} \nabla_2^2 P(t), \end{aligned} \tag{21}$$

and

$$\boldsymbol{L}_s \cdot [\boldsymbol{p} P(t)] = -\nabla_1 \cdot \left[ \frac{1}{\gamma} f_s \boldsymbol{p} P(t) \right] \tag{22}$$

accounts for the swim force.

To get an equation for $\phi$, we take the scalar product of 1 with Eq. (20), which gives

$$\partial_t \phi = L\phi + \frac{1}{d} \boldsymbol{L}_s \cdot \boldsymbol{\sigma}. \tag{23}$$

The scalar product of $\boldsymbol{p}$ with Eq. (20) gives an equation for $\boldsymbol{\sigma}$:

$$\partial_t \boldsymbol{\sigma} = -\tau^{-1} \boldsymbol{\sigma} + L\boldsymbol{\sigma} + \boldsymbol{L}_s \phi + \frac{2}{2+d} \boldsymbol{L}_s \cdot \boldsymbol{\omega} \tag{24}$$

where $\tau^{-1} = (d-1) D_r + \alpha$ is the inverse of the relaxation time of the $\boldsymbol{\sigma}$ mode, which is equal to the autocorrelation time of the orientation vector $\boldsymbol{p}$.

The scalar product of $\boldsymbol{Q}$ with Eq. (20) gives an equation for $\boldsymbol{\omega}$:

$$\partial_t \boldsymbol{\omega} = -\tau_\omega^{-1} \boldsymbol{\omega} + L\boldsymbol{\omega} + \boldsymbol{A} : \boldsymbol{L}_s \boldsymbol{\sigma} + \boldsymbol{L}_s \cdot \boldsymbol{\Upsilon}, \tag{25}$$

where $\tau_\omega^{-1} = 2dD_r + \alpha$ is the inverse of the relaxation time of the $\boldsymbol{\omega}$ mode, and

$$\boldsymbol{\Upsilon} = \frac{d}{\Omega_d} \frac{2}{2+d} \left\langle \boldsymbol{pQ}, \Theta\left(P(t)\right) \right\rangle, \tag{26}$$

involves higher order coefficients of the expansion in Eq. (6).

Equations (23), (24) and (25) are exact and form a hierarchy of equations. However, this hierarchy is not closed due to the $\Upsilon$ term in Eq. (25). Often the hierarchy is closed by assuming that the nematic order ($\boldsymbol{Q}$) in the system is negligible [5], or that the projection onto the higher order modes is zero [12]. Here we do not do this as $\boldsymbol{Q}$ is not small in general. However, as shown explicitly, below, on a course-grained level where one only considers the position of the dimer and not the positions of the two particles individually, it will turn out that the contribution to the flux from $\boldsymbol{Q}$ and $\Upsilon$ are of the order $\sim \nabla^3$ and can therefore be ignored.

### C. Elimination of the internal degree of freedom

Next use the following coordinate transformation:

$$\boldsymbol{R} = \frac{1}{1+q}\boldsymbol{r}_1 + \frac{q}{1+q}\boldsymbol{r}_2, \tag{27}$$

$$\boldsymbol{r}' = \boldsymbol{r}_1 - \boldsymbol{r}_2, \tag{28}$$

where $\boldsymbol{R}$ is the 'center-of-friction' coordinate, which we call the collective coordinate, and $\boldsymbol{r}'$ is the internal degree of freedom. The gradient with respect to the $\boldsymbol{R}$ coordinate is $\nabla$, and the gradient with respect to the $\boldsymbol{r}'$ coordinate is $\nabla'$. With this, the equation for the density [Eq. (23)] becomes

$$\begin{aligned}\partial_t\phi =& \frac{1}{1+q}\frac{T}{\gamma}\nabla^2\phi - \frac{1}{1+q}\frac{1}{d}\frac{1}{\gamma}\nabla\cdot(f_s\boldsymbol{\sigma}) \\ &- \nabla'\cdot\left[\frac{1}{\gamma}f_s\boldsymbol{\sigma} + \frac{1+q}{q}\frac{1}{\gamma}\boldsymbol{F}\phi - \frac{1+q}{q}\frac{T}{\gamma}\nabla'\phi\right].\end{aligned} \tag{29}$$

We are interested in the large scale behaviour of the system, so we want to know

$$\rho(\boldsymbol{R},t) = \int_V d^dr'\ \phi(\boldsymbol{R},\boldsymbol{r}',t), \tag{30}$$

which obeys

$$\partial_t\rho = -\nabla\cdot\boldsymbol{J}, \tag{31}$$

where $\boldsymbol{J} = \boldsymbol{J}_D + \boldsymbol{J}_\sigma$,

$$\boldsymbol{J}_D = -\frac{1}{1+q}\frac{T}{\gamma}\nabla\rho \tag{32}$$

is the flux due to passive diffusion, and

$$\boldsymbol{J}_\sigma = \frac{1}{1+q}\frac{1}{d\gamma}\int_V d^dr'\ f_s\boldsymbol{\sigma}, \tag{33}$$

is the flux due to the activity. In the new coordinates, the equations for $\boldsymbol{p}$ and $\boldsymbol{\omega}$ become,

$$\begin{aligned}(1+\tau\partial_t)\boldsymbol{\sigma} =& -\left(\frac{1}{1+q}\nabla + \nabla'\right)\frac{\tau}{\gamma}(f_s\phi) \\ &- \frac{1+q}{q}\frac{\tau}{\gamma}\nabla'\cdot(\boldsymbol{F}\boldsymbol{\sigma}) \\ &+ \tau\left(\frac{1}{1+q}\nabla^2 + \frac{1+q}{q}\nabla'^2\right)\boldsymbol{\sigma} \\ &- \frac{2}{2+d}\frac{\tau}{\gamma}\left(\frac{1}{1+q}\nabla + \nabla'\right)\cdot(f_s\boldsymbol{\omega}),\end{aligned} \tag{34}$$

$$(1+\tau_\omega\partial_t)\boldsymbol{\omega} = -\tau_\omega\nabla\cdot M_{\boldsymbol{R}} - \tau_\omega\nabla'\cdot M_{\boldsymbol{r}'}. \tag{35}$$

The form of the tensors $M_{\boldsymbol{R}}$ and $M_{\boldsymbol{r}'}$ and not used because these terms are only used to show that they have a contribution to $\rho$ of the order of $\sim \mathcal{O}\left(\nabla^3\right)$ and can therefore be neglected.

The density $\rho$ obeys a continuity equation, is therefore locally conserved and relaxes on a time scale $\sim \mathcal{O}\left((\nabla)^{-1}\right)$. The $\boldsymbol{p}$ and $\boldsymbol{\omega}$ modes relax on a time scale $\tau$ and $\tau_\omega$, respectively. So $\rho$ can be identified as the slow mode, $\boldsymbol{p}$ and $\boldsymbol{\omega}$ are the fast modes; therefore, one can set the time derivatives in the two previous equations to zero.

Furthermore, we are interested in the limit where the gradient of the swim force is small compared to the separation between the two particles and small compared to the persistence length of the active particle ($\tau f_s/\gamma$). The expansion coefficients are functions of $\boldsymbol{R}$ and $\boldsymbol{r}'$. Gradients in $\boldsymbol{R}$ of these functions are of the same order as gradients of the swim force and are therefore small. Gradients in $\boldsymbol{r}'$ of the expansion coefficients, however, are not small, but these can be moved around in the integral by integration by parts and turned into gradients with respect to $\boldsymbol{R}$ by using $\nabla' v = \nabla' v(\boldsymbol{R}+\frac{q}{1+q}\boldsymbol{r}') = \frac{q}{1+q}\nabla v$. We will neglect terms $\sim \mathcal{O}\left(\nabla^3\right)$ in Eq. (31), which means that we neglect terms $\sim \mathcal{O}\left(\nabla^2\right)$ when calculating $\boldsymbol{J}_\sigma$.

We can than use Eq. (34) to calculate $\boldsymbol{J}_\sigma$:

$$\begin{aligned}\boldsymbol{J}_\sigma =& -\frac{1}{(1+q)^2}\frac{1}{d\gamma^2}\int_V d^dr'\ \tau f_s\nabla(f_s\phi) \\ &- \frac{1}{1+q}\frac{1}{d\gamma^2}\int_V d^dr'\ \tau f_s\nabla'(f_s\phi) \\ &- \frac{1}{q}\frac{1}{d\gamma^2}\int_V d^dr'\ \tau f_s\nabla'\cdot(\boldsymbol{F}\boldsymbol{\sigma}) \\ &+ \frac{1}{1+q}\frac{1}{d\gamma}\int_V d^dr' \\ &\quad \tau f_s\left(\frac{1}{1+q}\nabla^2 + \frac{1+q}{q}\nabla'^2\right)\boldsymbol{\sigma} \\ &+ \frac{2}{2+d}\frac{1}{1+q}\frac{\tau_\omega}{d\gamma^2}\int_V d^dr' \\ &\quad f_s\left(\frac{\nabla}{1+q} + \nabla'\right)\cdot(f_s\boldsymbol{\omega}).\end{aligned} \tag{36}$$

In the last two integrals, one can use integration by parts to make the $\nabla'$'s (also the ones in $\boldsymbol{\omega}$, see Eq. (35)) act on

$f_s$, and $\nabla' f_s \propto \nabla f_s$ to show that the last two integrals are second order in $\nabla$ and can be neglected. For the second and third integral we use integration by parts. This gives

$$\begin{aligned} \boldsymbol{J}_\sigma =& -\frac{1}{(1+q)^2}\frac{\tau}{d\gamma^2}\int_V d^dr'\ f_s\nabla(f_s\phi) \\ &+ \frac{q}{(1+q)^2}\frac{\tau}{d\gamma^2}\int_V d^dr'\ \phi f_s\nabla f_s \\ &+ \frac{1}{1+q}\frac{\tau}{d\gamma^2}I, \end{aligned} \tag{37}$$

where

$$I = \int_V d^dr'\ (\boldsymbol{F}\cdot\nabla f_s)\,\boldsymbol{\sigma}, \tag{38}$$

$$= -\frac{\tau}{\gamma}\int_V d^dr'\ \boldsymbol{F}\cdot(\nabla f_s) \nabla'\cdot\left(\mathbf{1}\phi f_s + \frac{1+q}{q}\boldsymbol{F}\sigma\right) \tag{39}$$

$$= \frac{\tau}{\gamma}\int_V d^dr'\ \left(\mathbf{1}\phi f_s + \frac{1+q}{q}\sigma\boldsymbol{F}\right)\cdot \nabla'(\boldsymbol{F}\cdot\nabla f_s). \tag{40}$$

Next we use

$$\nabla'(\boldsymbol{F}\cdot\nabla f_s) = (\nabla'\boldsymbol{F})\cdot\nabla f_s + \mathcal{O}(\nabla^2 f_s), \tag{41}$$

and

$$\nabla'\boldsymbol{F} = -k\nabla'[(r'-l_0)\hat{\boldsymbol{r}}'] = -k\boldsymbol{A}, \tag{42}$$

with $\boldsymbol{A} = \hat{\boldsymbol{r}}'\hat{\boldsymbol{r}}' + (1-l_0/r')(\mathbf{1}-\hat{\boldsymbol{r}}'\hat{\boldsymbol{r}}')$, and $r' = |\boldsymbol{r}'|$ and $\hat{\boldsymbol{r}}' = \boldsymbol{r}'/r'$. Note that $\boldsymbol{F}\cdot\boldsymbol{A} = \boldsymbol{F}$. With this, $I$ becomes

$$\begin{aligned} I =& -\frac{\tau k}{\gamma}\int_V d^dr'\ \phi f_s\boldsymbol{A}\cdot\nabla f_s \\ &- \frac{1+q}{q}\frac{\tau k}{\gamma}\int_V d^dr'\ (\boldsymbol{F}\cdot\nabla f_s)\,\boldsymbol{\sigma}, \end{aligned} \tag{43}$$

$$= -\frac{\tau k}{\gamma}\int_V d^dr'\ \phi f_s\boldsymbol{A}\cdot\nabla f_s - \frac{1+q}{q}\frac{\tau k}{\gamma}I, \tag{44}$$

$$= -\frac{q\tau k/\gamma}{q+(1+q)\tau k/\gamma}\int_V d^dr'\ \phi f_s\boldsymbol{A}\cdot\nabla f_s. \tag{45}$$

With this Eq. (37) becomes

$$\begin{aligned} \boldsymbol{J}_\sigma =& -\frac{1}{(1+q)^2}\frac{\tau}{d\gamma^2}\int_V d^dr'\ f_s\nabla(f_s\phi) \\ &+ \frac{q}{(1+q)^2}\frac{\tau}{d\gamma^2}\int_V d^dr'\ \phi f_s\nabla f_s \\ &- \frac{1}{(1+q)^2}\frac{\tau}{d\gamma^2}\frac{q(1+q)\tau k/\gamma}{q+(1+q)\tau k/\gamma} \\ &\int_V d^dr'\ \phi f_s\ \boldsymbol{A}\cdot\nabla f_s. \end{aligned} \tag{46}$$

Next we consider two cases for the potential: First, a rigid bond modeled as a harmonic spring with infinite spring constant and a nonzero rest length. Second, a harmonic spring with zero rest length.

### 1. *Rigid bond*

If the force is infinitely strong, that is $k\to\infty$,

$$\lim_{k\to\infty}\frac{q(1+q)\tau k/\gamma}{q+(1+q)\tau k/\gamma} = q. \tag{47}$$

Furthermore, we can approximate $\phi(\boldsymbol{R},\boldsymbol{r}',t) \approx \rho(\boldsymbol{R},t)\delta(r'-l_0)l_0^{1-d}/\Omega_d$, because $r'\approx l_0$ as $k\to\infty$, and the deviation from a uniform distribution on a sphere (or circle for $d=2$) is proportional to gradients of the swim force and therefore contributes to the flux terms of the order $\sim\mathcal{O}\left(\nabla^2\right)$. With this approximation the first two integrals in Eq. (46) become

$$\begin{aligned} &-\frac{1}{(1+q)^2}\frac{\tau}{d\gamma^2}\int_V d^dr'\ f_s\nabla(f_s\phi) \\ &+ \frac{q}{(1+q)^2}\frac{\tau}{d\gamma^2}\int_V d^dr'\ \phi f_s\nabla f_s \\ =& -\frac{1}{(1+q)^2}\frac{\tau}{d\gamma^2}\left(f_s^2\nabla\rho - q\rho\frac{1}{2}\nabla f_s^2\right), \end{aligned} \tag{48}$$

where the swim force has been taken out of the integral because $f_s = f_s(\boldsymbol{r}_1) = f_s(\boldsymbol{R}+\boldsymbol{r}'q/(1+q)) = f_s(\boldsymbol{R}) + \mathcal{O}(\nabla f_s)$. The last integral in Eq. (46) becomes

$$\begin{aligned} &-\frac{q}{(1+q)^2}\frac{\tau}{d\gamma^2}\int_V d^dr'\ \phi f_s\ \boldsymbol{A}\cdot\nabla f_s \\ =& -\frac{q}{(1+q)^2}\frac{\tau}{2d\gamma^2}\rho f_s(\nabla f_s)\cdot\int_V d^dr'\ \frac{r'^{1-d}}{\Omega_d}\delta(r'-l_0)R, \\ =& -\frac{q}{(1+q)^2}\frac{\tau}{d\gamma^2}\rho f_s(\nabla f_s)\cdot\int d\Omega_d\frac{\hat{\boldsymbol{r}}'\hat{\boldsymbol{r}}'}{\Omega_d}, \\ =& -\frac{q}{(1+q)^2}\frac{\tau}{d\gamma^2}\rho\frac{1}{2d}\nabla f_s^2, \end{aligned} \tag{49}$$

where we used $\int d\Omega_d\hat{\boldsymbol{r}}'\hat{\boldsymbol{r}}' = \Omega_d\mathbf{1}/d$. With this, we find

$$\begin{aligned} \boldsymbol{J}_\sigma =& -\frac{1}{(1+q)^2}\frac{\tau}{d\gamma^2}f_s^2(\boldsymbol{R})\nabla\rho \\ &- \frac{\epsilon}{(1+q)^2}\frac{\tau}{d\gamma^2}\rho\frac{1}{2}\nabla f_s^2(\boldsymbol{R}), \end{aligned} \tag{50}$$

where

$$\epsilon = 1 - q\frac{d-1}{d}. \tag{51}$$

The total flux is

$$\boldsymbol{J} = \boldsymbol{J}_D + \boldsymbol{J}_\sigma, \tag{52}$$

$$\begin{aligned} =& -\frac{1}{1+q}\frac{T}{\gamma}\nabla\rho - \frac{1}{(1+q)^2}\frac{\tau}{d\gamma^2}f_s^2(\boldsymbol{R})\nabla\rho \\ &- \frac{\epsilon}{(1+q)^2}\frac{\tau}{d\gamma^2}\rho\frac{1}{2}\nabla f_s^2(\boldsymbol{R}), \end{aligned} \tag{53}$$

$$= \boldsymbol{V}(\boldsymbol{R})\rho - D(\boldsymbol{R})\nabla\rho, \tag{54}$$

where

$$D(\boldsymbol{R}) = \frac{1}{1+q}\frac{T}{\gamma} + \frac{1}{(1+q)^2}\frac{\tau}{d\gamma^2}f_s^2(\boldsymbol{R}), \tag{55}$$

is the space-dependent diffusion coefficient, and

$$\boldsymbol{V}(\boldsymbol{R}) = -\frac{1}{2}\epsilon\frac{1}{(1+q)^2}\frac{\tau}{d\gamma^2}\nabla f_s^2(\boldsymbol{R}), \tag{56}$$

$$= -\frac{1}{2}\epsilon\nabla D(\boldsymbol{R}), \tag{57}$$

is the drift velocity.

The flux-free steady-state solution for $\rho$ is

$$\rho \propto \left[1 + \frac{1}{1+q}\frac{\tau}{d\gamma T}f_s^2(\boldsymbol{R})\right]^{-\frac{1}{2}\epsilon}. \tag{58}$$

For $\epsilon = 0$ the density is flat and independent of the swim-force profile. This happens when $q$ is equal to

$$q_0 = \frac{d}{d-1} = \begin{cases} 3/2 & \text{for } d = 3, \\ 2 & \text{for } d = 2. \end{cases} \tag{59}$$

In the limit of highly mobile cargo, that is $q \to 0$, the density becomes

$$\rho \propto \left[1 + \frac{\tau}{d\gamma T}f_s^2(\boldsymbol{R})\right]^{-\frac{1}{2}}, \tag{60}$$

which is the density of a single active particle in a space dependent swim force [3, 13]

In the limit of high friction cargo ($q \to \infty$) the density becomes

$$\rho \propto \exp\left[\frac{d-1}{2d}\frac{\tau}{d\gamma T}f_s^2(\boldsymbol{R})\right]. \tag{61}$$

Whether the drift velocity (Eq. (57)) is up or down the swim force gradient, depends on the sign of $\epsilon$: when $\epsilon > 0$ ( $q < d/(d-1)$) the drift velocity is down the swim force gradient, which corresponds to antichemotaxis; when $\epsilon < 0$ ( $q > d/(d-1)$) the drift velocity is up the swim force gradient, which corresponds to chemotaxis. For the infinitely strong potential with nonzero rest length, $\epsilon = 0$ for $q = d/d-1$, and decreases with increasing $q$, so with increasing friction of the cargo, the chemotactic behaviour increases. The maximum drift velocity is obtained for

$$q_{max} = \frac{3d-1}{d-1} = \begin{cases} 5 & \text{for } d = 2, \\ 4 & \text{for } d = 3. \end{cases} \tag{62}$$

#### 2. *Harmonic force with zero rest length*

We are interested in the range where the separation between the two particles is small compared to the gradients of the swim force.

Because the separation between the two particles is assumed to be small compared to the gradients in the swim force, for the first two integral in Eq. (46), we can use $\phi(\boldsymbol{R}, \boldsymbol{r}', t) \approx \rho(\boldsymbol{R}, t)\delta^{(3)}(\boldsymbol{r}')$. This, together with $\boldsymbol{A}(l_0 = 0) = \boldsymbol{1}$, gives

$$\begin{aligned}\boldsymbol{J}_\sigma = &-\frac{1}{(1+q)^2}\frac{\tau}{d\gamma^2}f_s^2(\boldsymbol{R})\nabla\rho \\ &-\frac{\epsilon}{(1+q)^2}\frac{\tau}{d\gamma^2}\rho\frac{1}{2}\nabla f_s^2(\boldsymbol{R}),\end{aligned} \tag{63}$$

where

$$\epsilon = 1 - \frac{q^2}{q + (1+q)\frac{\tau k}{\gamma}}. \tag{64}$$

The total flux and steady-state density are the same as for the rigid bond (Eq. (54) and Eq. (58)), but with $\epsilon$ given by the previous equation. Note that in the limit $k \to \infty$, $\epsilon = 1$, and the dimer behaves like a single active particle with a increased friction constant. The limit $k = 0$ is not possible, as it violates the assumption that the separation between the two particles is small compared to the gradients in the swim force. The value of $q$ for which the density is flat, obtained by equating $\epsilon$ to zero, is

$$q_0 = \frac{1}{2}\left(1 + \frac{\tau k}{\gamma}\right) + \frac{1}{2}\sqrt{\left(1 + \frac{\tau k}{\gamma}\right)^2 + 4\frac{\tau k}{\gamma}}. \tag{65}$$

The small $q$ limit the dimer behaves the same as a single active particle with an increased friction constant, and the steady-state density is the same as for the rigid bond (Eq. (60)). In the limit of large $q$, the steady-state density becomes

$$\rho(\boldsymbol{R}) \propto \exp\left[\frac{1}{1 + \frac{\tau k}{\gamma}}\frac{\tau}{2d\gamma T}f_s^2(\boldsymbol{R})\right] \tag{66}$$

### D. The Born-Oppenheimer approximation

Here we derive the steady-state density in the limit $q \to \infty$. Only the derivation for the dimer with a rigid bond is shown; the derivation for the harmonic potential is similar. In this limit, the dynamics of the cargo particle are much slower than the dynamics of the active particle. Due to this separation of time scales, we can use a Born-Oppenheimer approximation [14]. In this approximation, we calculate the average force that the active particle exerts on the passive cargo particle that is fixed at the origin. To be more precise, we start by calculating the average force on the active particle due to a fixed potential $U$. The equations for an active particle in a potential are

$$\partial_t \boldsymbol{r}_1 = \frac{1}{\gamma}\boldsymbol{F} + f_s(\boldsymbol{r}_1)\boldsymbol{p} + \sqrt{2T/\gamma}\boldsymbol{\xi}, \tag{67}$$

$$\partial_t \boldsymbol{p} = \sqrt{2D_r}\boldsymbol{p} \times \boldsymbol{\eta} + \text{tumbling}, \tag{68}$$

where $\boldsymbol{F} = -\nabla_1 U(\boldsymbol{r}_1)$ with $U(\boldsymbol{r}_1) = \frac{1}{2}k(r_1 - l_0)^2$. The corresponding FPE is

$$\begin{aligned}\partial_t W(\boldsymbol{r}_1, \boldsymbol{p}, t) =& -\nabla_1 \cdot \left[\frac{1}{\gamma}\boldsymbol{F}W - \frac{T}{\gamma}\nabla_1 W\right] \\ & -\nabla_1 \cdot \left[\frac{1}{\gamma} f_s \boldsymbol{p} W\right] + D_r \boldsymbol{\mathcal{R}}^2 W \\ & -\alpha W + \alpha\phi,\end{aligned} \tag{69}$$

where the last two lines account for the tumbling and

$$\phi(\boldsymbol{r}_1, t) = \int d\Omega_d W(\boldsymbol{r}_1, \boldsymbol{p}(\Omega_d), t). \tag{70}$$

The probability density $W$ can be expanded

$$W(t) = \phi + \boldsymbol{\sigma}\cdot\boldsymbol{p} + \boldsymbol{\omega} : \boldsymbol{Q} + \Theta\left(W(t)\right), \tag{71}$$

where $\phi$, $\boldsymbol{\sigma}$ and $\boldsymbol{\omega}$ are functions of $\boldsymbol{r}_1$ and $t$. The equation for the coefficients are obtained, as before, by taking scalar products. The equation for $\phi$ is

$$\partial_t \phi = -\nabla_1 \cdot \boldsymbol{J}, \tag{72}$$

where

$$\boldsymbol{J} = \frac{1}{\gamma}\boldsymbol{F}\phi - \frac{T}{\gamma}\nabla_1\phi + \frac{1}{d\gamma} f_s \boldsymbol{\sigma}. \tag{73}$$

The equation for $\boldsymbol{\sigma}$ is

$$\begin{aligned}\partial_t \boldsymbol{\sigma} =& -\tau^{-1}\boldsymbol{\sigma} - \nabla_1 \cdot \left[\frac{1}{\gamma}\boldsymbol{F}\boldsymbol{\sigma} - \frac{T}{\gamma}\nabla_1 \boldsymbol{\sigma}\right] \\ & -\nabla_1\left[\frac{1}{\gamma} f_s \phi\right] - \nabla_1 \cdot \left[\frac{1}{\gamma} f_s \boldsymbol{\omega}\right].\end{aligned} \tag{74}$$

The equation for $\boldsymbol{\omega}$ is

$$\begin{aligned}\partial_t \boldsymbol{\omega} =& -\nabla_1 \cdot \left[\frac{1}{\gamma}\boldsymbol{F}\boldsymbol{\omega} - \frac{T}{\gamma}\nabla_1 \boldsymbol{\omega}\right] \\ & -\frac{2+d}{d}\nabla_1\left[\frac{1}{\gamma} f_s \boldsymbol{\sigma}\right] - \nabla_1 \cdot \left[\frac{1}{\gamma} f_s \Upsilon\right],\end{aligned} \tag{75}$$

where $\Upsilon = \frac{\Omega}{d}\frac{2}{2+d}\langle \boldsymbol{p}\boldsymbol{Q}, \Theta\rangle$, is the projection onto higher order harmonics.

The average force on the active particle due to the potential is

$$\boldsymbol{F}_{avg} = \int d^d r\ \boldsymbol{F}(\boldsymbol{r}_1)\phi(\boldsymbol{r}_1), \tag{76}$$

where $\phi$ is the steady-state density. In steady state, the flux is zero, and Eq. (73) can be used to rewrite the expression for the average force:

$$\boldsymbol{F}_{avg} = \int d^d r\ T\nabla_1\phi - \int d^d r\ \gamma\frac{1}{d\gamma} f_s \boldsymbol{\sigma}. \tag{77}$$

The first integral is zero because $\phi(r = \infty) = 0$, and $\boldsymbol{\sigma}$ in the second integral can be replaced by the expression in Eq. (74) with $\partial_t \boldsymbol{\sigma} = 0$. This gives

$$\begin{aligned}\boldsymbol{F}_{avg} =& \frac{1}{d\gamma}\int d^d r\ f_s \tau \nabla_1 (f_s \phi) \\ & + \frac{1}{d\gamma}\int d^d r\ f_s \tau \nabla_1 \cdot (\boldsymbol{F}\boldsymbol{\sigma}) \\ & - \frac{1}{d\gamma} T \int d^d r\ f_s \tau \nabla_1^2 \boldsymbol{\sigma} \\ & + \frac{1}{d\gamma}\int d^d r\ f_s \tau \nabla_1 \cdot \boldsymbol{\omega}.\end{aligned} \tag{78}$$

The third and fourth integrals are second order in $\nabla_1$ and can be neglected. This can be seen by integrating by parts twice (there is also a $\nabla_1$ in $\boldsymbol{\omega}$). For the first two integrals we use integration by parts. This gives

$$\begin{aligned}\boldsymbol{F}_{avg} =& -\frac{\tau}{d\gamma}\int d^d r\ \phi f_s \nabla_1 f_s \\ & - \frac{\tau}{d\gamma}\int d^d r\ \boldsymbol{\sigma}\boldsymbol{F}\cdot\nabla_1 f_s, \qquad (79) \\ =& -\frac{\tau}{d\gamma}\int d^d r\ \phi f_s \nabla_1 f_s - \frac{\tau}{d\gamma} I, \qquad (80)\end{aligned}$$

where

$$\begin{aligned}I \equiv& \int d^d r\ \boldsymbol{\sigma}\boldsymbol{F}\cdot\nabla_1 f_s, \qquad (81) \\ =& -\frac{\tau}{\gamma}\int d^d r\ \boldsymbol{F}\cdot(\nabla_1 f_s)\left[\nabla_1\cdot(F\boldsymbol{\sigma}) + \nabla_1(f_s\phi)\right], \qquad (82) \\ =& \frac{\tau}{\gamma}\int d^d r\ \left[\boldsymbol{\sigma}\boldsymbol{F} + f_s\phi\boldsymbol{1}\right]\cdot\nabla_1(\boldsymbol{F}\cdot\nabla_1 f_s), \qquad (83)\end{aligned}$$

where in the second line we ignored terms $\mathcal{O}\left(\nabla_1^2 f_s, (\nabla_1 f_s)^2\right)$, and used integration by parts to go to the last line. Next we use again

$$\nabla_1\left(\boldsymbol{F}\cdot\nabla_1 f_s\right) = (\nabla_1\boldsymbol{F})\cdot\nabla_1 f_s + \mathcal{O}\left(\nabla_1^2 f_s\right), \tag{84}$$

and

$$\begin{aligned}\nabla_1\boldsymbol{F} =& -k\nabla_1\left[(r - l_0)\hat{\boldsymbol{r}}_1\right], \qquad (85) \\ =& -k\boldsymbol{A}, \qquad (86)\end{aligned}$$

where $\boldsymbol{A} \equiv \hat{\boldsymbol{r}}_1\hat{\boldsymbol{r}}_1 + \left(1 - \frac{l_0}{r_1}\right)(\boldsymbol{1} - \hat{\boldsymbol{r}}_1\hat{\boldsymbol{r}}_1)$ , $r_1 = |\boldsymbol{r}_1|$, and $\hat{\boldsymbol{r}}_1 = \boldsymbol{r}_1/r_1$. With this $I$ becomes

$$\begin{aligned}I =& -\frac{\tau k}{\gamma}\int d^d r\ \phi f_s \boldsymbol{A}\cdot\nabla_1 f_s - \frac{\tau k}{\gamma}\int d^d r\ \boldsymbol{\sigma}\boldsymbol{F}\cdot f_s, \qquad (87) \\ =& -\frac{\tau k}{\gamma}\int d^d r\ \phi f_s \boldsymbol{A}\cdot\nabla_1 f_s - \frac{\tau k}{\gamma} I, \qquad (88) \\ =& -\frac{\tau k/\gamma}{1 + \tau k/\gamma}\int d^d r\ \phi f_s \boldsymbol{A}\cdot\nabla_1 f_s, \qquad (89)\end{aligned}$$

where we used $\boldsymbol{F}\cdot\boldsymbol{A} = \boldsymbol{F}$.

The average force then becomes

$$\boldsymbol{F}_{avg} = -\frac{\tau}{d\gamma}\int d^d r\ \phi f_s \nabla_1 f_s + \frac{\tau k/\gamma}{1+\tau k/\gamma}\frac{\tau}{d\gamma}\int d^d r\ \phi f_s \boldsymbol{A}\cdot\nabla_1 f_s. \tag{90}$$

For an infinitely stiff potential $k \to \infty$, and

$$\lim_{k\to\infty}\frac{\tau k/\gamma}{1+\tau k/\gamma} = 1, \tag{91}$$

and we can approximate $\phi(\boldsymbol{r}_1) \approx \frac{1}{\Omega_d} r_1^{1-d}\delta(r_1 - l_0)$, because the deviation from an uniform distribution is proportional to gradients in the swim force, so it contributes to the second order term in the average force. Furthermore, if gradients in the swim force are small compared to $r$, the terms with swim force can be taken out of the integral, as the error is $\sim \mathcal{O}(\nabla)$. In this limit, the average force becomes

$$\boldsymbol{F}_{avg} = -\frac{\tau}{2d\gamma}\left[\nabla_1 f_s^2\right]_{\boldsymbol{r}_1=0}\int d^d r\ \phi + \frac{\tau}{2d\gamma}\left[\nabla_1 f_s^2\right]_{\boldsymbol{r}_1=0}\cdot\int d\Omega_d\ \frac{1}{\Omega_d}\hat{\boldsymbol{r}}_1\hat{\boldsymbol{r}}_1, \tag{92}$$

$$= -\frac{d-1}{d}\frac{\tau}{2d\gamma}\left[\nabla_1 f_s^2\right]_{\boldsymbol{r}_1=0}, \tag{93}$$

where we used $\int d\Omega_d\ \hat{\boldsymbol{r}}_1\hat{\boldsymbol{r}}_1 = \mathbf{1}\Omega_d/d$. Note that the average force on the cargo particle is $-\boldsymbol{F}_{avg}$.

Now consider the case where the position of the passive cargo particle is no fixed to the origin, but it moves slowly compared to the active particle. Then, if the cargo particle is at position $\boldsymbol{r}_2$, it experiences an effective force

$$\boldsymbol{F}_{eff} = \frac{d-1}{d}\frac{\tau}{2d\gamma}\nabla_2 f_s^2(\boldsymbol{r}_2), \tag{94}$$

which is minus $\boldsymbol{F}_{avg}$ with the origin shifted to the location of the cargo particle. The equation of motion of a passive Brownian particle with friction $q\gamma$ diffusing in a force field $\boldsymbol{F}_{eff}$ is

$$\partial_t \boldsymbol{r}_2 = \frac{1}{q\gamma}\boldsymbol{F}_{eff} + \sqrt{2T/q\gamma}\chi. \tag{95}$$

The corresponding FPE is

$$\partial_t \rho(\boldsymbol{r}_2, t) = -\nabla_2\cdot\boldsymbol{J}, \tag{96}$$

$$\boldsymbol{J} = \frac{1}{q\gamma}\boldsymbol{F}_{eff}\rho - \frac{T}{q\gamma}\nabla_2\rho. \tag{97}$$

Equating the flux to zero gives the steady-state density distribution:

$$\rho(\boldsymbol{r}_2) \propto \exp\left[\frac{d-1}{d}\frac{\tau}{2d\gamma T}f_s^2(\boldsymbol{r}_2)\right], \tag{98}$$

which is the same as Eq. (61). Note that to calculate the effective force ( Eq. (94)) and the flux (Eq. (97)) in this limit it is not necessary to calculate the steady-state density of an active particle in a fixed potential, which is a difficult problem on its own [4, 15]

### E. Average position of the dimer

In this section we show the derivation of the average position of the dimer in a box with length $L$. This is the theory shown in Fig. 3 in the main text. The simulations were done with a WCA potential for the walls. Here we ignore the details of the interaction of the dimer with the walls and model the walls as zero-flux boundary condition at the walls. The average postion of the dimer in the box is

$$\bar{R} = \int_{-L/2}^{L/2} dR\ R\rho(R,t). \tag{99}$$

The time derivative of this is

$$\partial_t \bar{R} = -\int_{-L/2}^{L/2} dR\ R\partial_R J(R,t), \tag{100}$$

$$= \int_{-L/2}^{L/2} dR\ J(R,t), \tag{101}$$

where we used the zero-flux condition at the boundaries. If the system starts with a homogeneous bulk density $\rho_b$, and we substitute Eq. (54) for the flux, the time derivative at $t = 0$ becomes

$$\partial_t \bar{R}|_{t=0} = -\frac{1}{2}\epsilon\rho_b\int_{-L/2}^{L/2} dR\partial_R D, \tag{102}$$

$$= -\frac{1}{2}\frac{\epsilon}{(1+q)^2}\frac{\tau}{d\gamma^2}\rho_b\int_{-L/2}^{L/2} dR\partial_R f_s^2. \tag{103}$$

The most important feature of this equation is

$$\partial_t \bar{R}|_{t=0} \propto \frac{\epsilon}{(1+q)^2}, \tag{104}$$

because indicates the dependence of $\partial_t \bar{R}|_{t=0}$ on $q$ independent of the swim-force profile or the geometry of the container.

For the case in Fig. 3 in the main text $f_s(R) = f_0\sqrt{R + L/2}$, with $f_0 = \sqrt{6}$. With this we get,

$$\partial_t \bar{R}|_{t=0} = -\frac{1}{2}\frac{\epsilon}{(1+q)^2}\frac{\tau}{d\gamma^2}f_0^2\rho_b L, \tag{105}$$

which is what is shown in Fig. 3 in the main text with $\rho_b = 1/L$ and $f_0 = \sqrt{6}$. In Fig. 1 we show a comparison between the theoretical prediction (Eq. (105) and a fit of (104) to simulation data.

## III. COMPARISON TO ACTIVE TEMPERATURE

Because Brownian particles coupled to different thermostats have shown interesting behaviour [16–19], we consider here a modification of the active-passive dimer model where the dimer is made up from a passive particle and a particle with a space-dependent temperature.

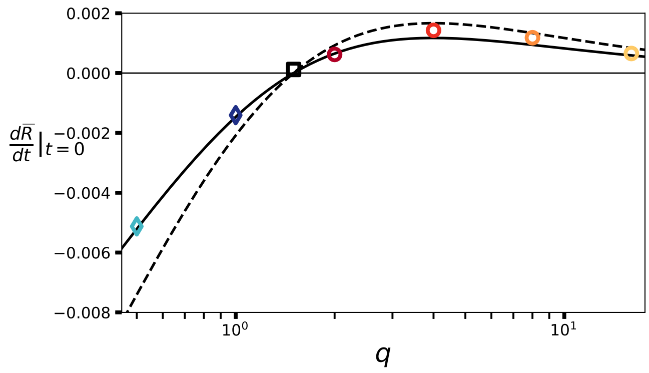


FIG. 1. The data (symbols) and theoretical prediction (dashed line, Eq. (105)) for the initial change in the average position of the dimer in the box. The solid shows Eq. (104) with the prefactor fitted to the data (as in Fig. 3 of the main text). Eventhough there is a discrepancy between the theoretical prediction and the simulation results for small values of $q$, the dendence on $q$ is accurately captured by the theory, as is indicated by the fit of Eq. (104) (sollid line). The mismatch between the theoretical prediction and the data is likely due to boundary effects in the simulation, which are ignored in the theory.

We do not consider this an approximate model for the active-passive dimer, where the activity is approximated by an effective temperature, as this concepts, although useful in some contexts, is not a well defined in general for far-from-equilibrium active-matter systems [20, 21].

The steady-state density of a single passive Brownian particle with a space-dependent temperature is [22]

$$\rho(\boldsymbol{r}_1) \propto \frac{1}{T(\boldsymbol{r}_1)}. \tag{106}$$

If a high temperature corresponds to a high activity, this corresponds to antichemotactic behaviour. If such a particle is bound to a heavy cargo particle, does it, as the active-passive dimer, become chemotactic?

If the persistence length of the active particle $\delta = \tau f_s/\gamma$ is constant all the integration by parts for $\nabla'$ in Eq. (36) yield zero, and up to first order in the gradient, $\boldsymbol{J}_\sigma$ becomes

$$\boldsymbol{J}_\sigma = -\frac{1}{(1+q)^2}\frac{1}{d\gamma^2}\int_V d^d r' \ \tau f_s \nabla(f_s\phi). \tag{107}$$

Using the same approximations as before yields for the total flux the same as Eq. (54) but with $\epsilon = 1$. The density of the dimer in this case is just that of a single active particle with friction $(1+q)\gamma$. So the only effect of increasing $q$ is that it increases the friction of the dimer, and there is no $q$ for which the dimer is chemotactic. Note that this holds for any $\delta$, not just in the "active temperature" limit.

This result can also be obtained from the Born-Oppenheimer approach. In this case all the integrals in Eq. (78) yield zero (this can be obtained by integrating by parts), and the average force is zero. So again, this shows that if the persistence length is constant the dimer acts as a single active particle with increased friction and does not exhibit chemotactic behaviour for any $q$.

In the limit $\delta \to 0$, a self-propelled particle with space-dependent swim force but constant persistence length becomes equivalent to a passive Brownian particle with temperature $T_{eff} = \frac{\tau f_s^2}{d\gamma} + T$ [2]. Therefore, the previous consideration shows that a dimer build from a passive Brownian particle in a temperature gradient attached to a passive cargo particle with a spatially independent temperature does not exhibit chemotactic behaviour for any value of $q$.

## IV. RUN-AND-TUMBLE DIMER IN ONE DIMENSION

### A. model

Because ABPs are not defined in one dimension, and RTPs in one dimension have a discrete orientation (either in the positive or in the negative direction), we show the derivation of the flux of the collective coordinate for this case separately. Because a fixed bond length in one dimension means that there is no internal degree of freedom, we only consider the case of a harmonic potential with different spring constants between the active and passive particle. The equations of motion are

$$\partial_t x_1 = \frac{1}{\gamma}F + \frac{1}{\gamma}f_s(x_1)p + \sqrt{2T/\gamma}\xi_1 \tag{108}$$

$$\partial_t x_2 = -\frac{1}{q\gamma}F + \sqrt{2T/\gamma}\xi_2, \tag{109}$$

where $x_1$ is the coordinate of the active particle with friction constant $\gamma$ and swim force $f_s$, $x_2$ is the coordinate of the passive cargo particle with friction constant $q\gamma$, $T$ is the temperature in units such that the Boltzmann constant is unity, and $\xi_1$ and $\xi_2$ are white noise with zero mean and autocorrelation $\langle\xi_1(t)\xi_1(t')\rangle = \langle\xi_2(t)\xi_2(t')\rangle = \delta(t-t')$. The orientation of the active particle is $p \in \{+1, -1\}$, which points either in the positive (right moving) or the negative (left moving) direction. With rate $\alpha$ the active particle randomizes its orientation (so it changes direction with rate $\alpha/2$). The force of the RTP on the passive cargo particle is $\boldsymbol{F} = -\partial_1 U$, where $U = -\frac{1}{2}k(x_1 - x_2)^2$. The corresponding FPE equation is

[23]

$$\partial_t\phi_R(t) =-\partial_1\left[\,v\phi_R(t)+\frac{1}{\gamma}F\phi_R(t)-\frac{T}{\gamma}\partial_1\phi_R(t)\right]$$
$$-\partial_2\left[-\frac{1}{q\gamma}F\phi_R(t)-\frac{T}{q\gamma}\partial_2\phi_R(t)\right]$$
$$-\frac{1}{2}\alpha\phi_R(t)+\frac{1}{2}\alpha\phi_L(t), \tag{110}$$
$$\partial_t\phi_L(t) =-\partial_1\left[-v\phi_L(t)+\frac{1}{\gamma}F\phi_L(t)-\frac{T}{\gamma}\partial_1\phi_L(t)\right]$$
$$-\partial_2\left[-\frac{1}{q\gamma}F\phi_L(t)-\frac{T}{q\gamma}\partial_2\phi_L(t)\right]$$
$$+\frac{1}{2}\alpha\phi_R(t)-\frac{1}{2}\alpha\phi_L(t), \tag{111}$$

where $\phi_R(t)=\phi_R(x_1,x_2,t)$ ($\phi_L(t)=\phi_L(x_1,x_2,t)$) is the probability density of a right (left) moving RTP at $x_1$ and a cargo particle at $x_2$.

Next we perform the same steps as in the two or three dimensional case. First we transfrom the equations using

$$\phi(t)=\phi_R(t)+\phi_L(t), \tag{112}$$
$$\sigma(t)=\phi_R(t)-\phi_L(t), \tag{113}$$

where $\phi(t)=\phi(x_1,x_2,t)$ is the density and $\sigma(t)=\sigma(x_1,x_2,t)$ is the excess of dimers with a right moving RTP. The equation density is

$$\partial_t\phi(t) =-\partial_1\left[v\sigma(t)+\frac{1}{\gamma}F\phi(t)-\frac{T}{\gamma}\partial_1\phi\right]$$
$$-\partial_2\left[-\frac{1}{q\gamma}F\phi(t)-\frac{T}{q\gamma}\partial_2\phi\right], \tag{114}$$

and

$$\partial_t\sigma(t) =-\alpha\sigma(t)$$
$$-\partial_1\left[v\phi(t)+\frac{1}{\gamma}F\sigma(t)-\frac{T}{\gamma}\partial_1\sigma\right]$$
$$-\partial_2\left[-\frac{1}{q\gamma}F\sigma(t)-\frac{T}{q\gamma}\partial_2\sigma\right]. \tag{115}$$

We use the same coordinate transformation as before:

$$X=\frac{1}{1+q}x_1+\frac{q}{1+q}x_2, \tag{116}$$
$$x'=x_1-x_2. \tag{117}$$

In these coordinates, the equations for $\phi$ and $\sigma$ become

$$\partial_t\phi(t) =-\frac{1}{1+q}\frac{1}{\gamma}\partial_X\left[f_s\sigma-T\partial_X\phi\right]$$
$$-\frac{1}{\gamma}\partial_{x'}\left[f_s\sigma+\frac{1+q}{q}F\phi-\frac{1+q}{q}T\partial_{x'}\phi\right], \tag{118}$$

$$\partial_t\sigma(t) =-\alpha\sigma-\frac{1}{1+q}\frac{1}{\gamma}\partial_X\left[f_s\phi-T\partial_X\sigma\right]$$
$$-\frac{1}{\gamma}\partial_{x'}\left[f_s\phi+\frac{1+q}{q}F\sigma-\frac{1+q}{q}T\partial_{x'}\sigma\right]. \tag{119}$$

Note that, in contrast with the two or three-dimensional cases (Eqs. (23) and (24)), the set of equations for $\phi$ and $\sigma$ is exact and closed.

## B. coarse graining the RTP dimer

Because we are interested in the large scale behaviour of the system, we want to know

$$\rho(X,t)=\int_{-\infty}^{\infty}dx'\ \phi(X,x',t), \tag{120}$$

which obeys

$$\partial_t\rho=-\partial_X J, \tag{121}$$

where $J=J_D+J_\sigma$,

$$J_D=-\frac{1}{1+q}\frac{T}{\gamma}\partial_X\rho \tag{122}$$

is the flux due to passive diffusion, and

$$J_\sigma=\frac{1}{1+q}\frac{1}{\gamma}\int_{-\infty}^{\infty}dx'\ f_s\sigma \tag{123}$$

is the flux due to the activity. The density obeys a continuity equation (Eq. (120)), so is locally conserved and relaxes on a time scale of the order $\sim\mathcal{O}\left((\partial_X)^{-1}\right)$. From Eq. (118) it follows that $\sigma$ relaxes on a time scale $1/\alpha$. So, as in the three dimensional case, $\rho$ can be identified as the slow degree of freedom and $\sigma$ as the fast degree of freedom; one can therefore neglect the time derivative in Eq. (119). Derivatives with respect to $X$ of $\rho$ and $\sigma$ are of the same order as $\partial f_s/\partial X$, which is small. Derivatives with respect to $x'$ of $\rho$ and $\sigma$ are not small, but the can be turned into derivatives with respect to $X$ by integration by parts and using $\partial_{x'}f_s=\partial_{x'}f_s(X+\frac{q}{1+q}x')=\frac{q}{1+q}\partial_X f_s$. Because derivatives with respect to $X$ are small, we neglect terms of the order $\mathcal{O}\left(\partial_X^3\right)$ in Eq. (120), which means we can neglect terms of the order $\mathcal{O}\left(\partial_X^2\right)$ in Eq. (123).

Using Eq. (119) and $\partial_t\sigma\approx 0$ to replace $\sigma$ in Eq. (123), we find

$$J_\sigma =\frac{1}{(1+q)^2}\frac{T}{\gamma^2\alpha}\int_{-\infty}^{\infty}dx'\ f_s\partial_X^2\sigma$$
$$-\frac{1}{(1+q)^2}\frac{1}{\gamma^2\alpha}\int_{-\infty}^{\infty}dx'\ f_s\partial_X\left(f_s\phi\right)$$
$$-\frac{1}{1+q}\frac{1}{\gamma^2\alpha}\int_{-\infty}^{\infty}dx'\ f_s\partial_{x'}\left(f_s\phi\right)$$
$$-\frac{1}{q}\frac{1}{\gamma^2\alpha}\int_{-\infty}^{\infty}dx'\ f_s\partial_{x'}\left(F\sigma\right)$$
$$-\frac{1}{q}\frac{T}{\gamma^2\alpha}\int_{-\infty}^{\infty}dx'\ f_s\partial_{x'}^2\sigma. \tag{124}$$

The first integral can be ignored because it is second order in derivatives with respect to $X$. The same holds for

the last integral because one can integrate by parts twice. For the second and third integral we use integration by parts. This gives

$$\begin{aligned} J_\sigma =& -\frac{1}{(1+q)^2}\frac{1}{\gamma^2\alpha}\int_{-\infty}^{\infty} dx'\ f_s\partial_X\left(f_s\phi\right) \\ &+\frac{q}{(1+q)^2}\frac{1}{\gamma^2\alpha}\int_{-\infty}^{\infty} dx'\ \phi f_s\partial_X f_s \\ &+\frac{1}{1+q}\frac{1}{\gamma^2\alpha}I, \end{aligned} \tag{125}$$

where

$$I \equiv \int_{-\infty}^{\infty} dx'\ \sigma F\partial_X f_s. \tag{126}$$

Using Eq. (119) again to replace $\sigma$ and ignoring second order derivatives with respect to $X$, we find

$$I = -\frac{1}{\alpha\gamma}\int_{-\infty}^{\infty} dx'\ F(\partial_X f_s)\partial_{x'}\left[f_s\phi+\frac{1+q}{q}F\sigma\right], \tag{127}$$

$$=\frac{1}{\alpha\gamma}\int_{-\infty}^{\infty} dx'\ \partial_{x'}\left[F(\partial_X f_s)\right]\left[f_s\phi+\frac{1+q}{q}F\sigma\right]. \tag{128}$$

The force is $F=-kx'$, so $\partial_{x'}\left[F(\partial_X f_s)\right] = -k\partial_X f_s + \mathcal{O}(\partial_X^2 f_s)$. With this, $I$ becomes

$$\begin{aligned} I =& -\frac{k}{\alpha\gamma}\int_{-\infty}^{\infty} dx'\ \phi f_s\partial_X f_s \\ &-\frac{k}{\alpha\gamma}\frac{1+q}{q}\int_{-\infty}^{\infty} dx'\ \sigma F\partial_X f_s, \end{aligned} \tag{129}$$

$$= -\frac{k}{\alpha\gamma}\int_{-\infty}^{\infty} dx'\ \phi f_s\partial_X f_s - \frac{k}{\alpha\gamma}\frac{1+q}{q}I, \tag{130}$$

$$= -\frac{q\frac{k}{\alpha\gamma}}{q+(1+q)\frac{k}{\alpha\gamma}}\int_{-\infty}^{\infty} dx'\ \phi f_s\partial_X f_s. \tag{131}$$

With the approximation $\phi(X,x',t)\approx\rho(X,t)\delta(x')$ and the result for $I$, $J_\sigma$ becomes

$$\begin{aligned} J_\sigma =& -\frac{1}{(1+q)^2}\frac{1}{\gamma^2\alpha}f_s^2(X)\partial_X\rho \\ &-\frac{1}{(1+q)^2}\frac{1}{\gamma^2\alpha}\frac{1}{2}\epsilon\rho\partial_X f_s^2(X), \end{aligned} \tag{132}$$

where

$$\epsilon = 1-\frac{q^2}{q+(1+q)\frac{k}{\gamma\alpha}}. \tag{133}$$

The total flux is

$$J = J_D + J_\sigma \tag{134}$$

$$= V(X)\rho - D(X)\partial_X\rho, \tag{135}$$

where

$$D(X) = \frac{1}{1+q}\frac{T}{\gamma} + \frac{1}{(1+q)^2}\frac{1}{\gamma^2\alpha}f_s^2(X) \tag{136}$$

is the space-dependent diffusion constant, and

$$V(X) = -\frac{1}{2}\epsilon\partial_X D(X) \tag{137}$$

is the drift velocity. The zero-flux steady-state density is

$$\rho(X) \propto \left[1+\frac{1}{1+q}\frac{1}{\gamma T\alpha}f_s^2(X)\right]^{-\frac{1}{2}\epsilon}. \tag{138}$$

Note that this is the same as the three dimensional case (Eq. (58) and $\epsilon$ shown in Eq. (64)) with $d=1$ and $\tau = 1/\alpha$, the autocorrelation time of the orientation of a one-dimensional RTP.

### C. numerical solution

Equations (118) and (119) can be solved numerically by a first order discretization of the space and time coordinates. Because these equations are exact, the numerical solution can be used to test the theoretical prediction for the steady-state density distribution Eq. (138), as well as explore interparticle potentials for which there is no theoretical prediction.

### D. results

All results are shown here are for $\gamma = 1$, $T = 1$, $k_b = 1$ and $\alpha = 40$ (so $\tau = 1/40$). Fig. 2 shows the steady-state density of dimers with harmonic potential for different friction of the cargo particle. The behaviour is qualitatively the same as the of a three-dimensional dimer with a fixed bond: the dimer is chemotactic if the cargo has a large friction, and is anti-chemotactic if the cargo has a small friction.

If the spring constant $k$ increases, the active particle is no longer able to explore the neighbourhood of the passive cargo particle and can therefore no longer sense the gradient in the swim force, which results in a decrease in the chemotaxis (see Fig. 3). The chemotactic behaviour is most pronounced in case of the weakest potential; however, the limit $k\to 0$ is not possible, as it violates the assumption that the separation between the active particle and the cargo particle is small compared to gradients of the swim force.

The theoretical analysis focused on a harmonic potential or a potential representing a fixed bond (only in two and three dimensions). To show that the transition from anti-chemotaxis to chemotaxis as the friction of the cargo increases is general, we consider the following potential:

$$U(x_1,x_2) = \begin{cases} 0 & \text{if} \quad |x_1-x_2| < l_0, \\ \infty & \text{else.} \end{cases} \tag{139}$$

This potential corresponds to a active particle and a cargo particle bound by a rope, so the active particle can

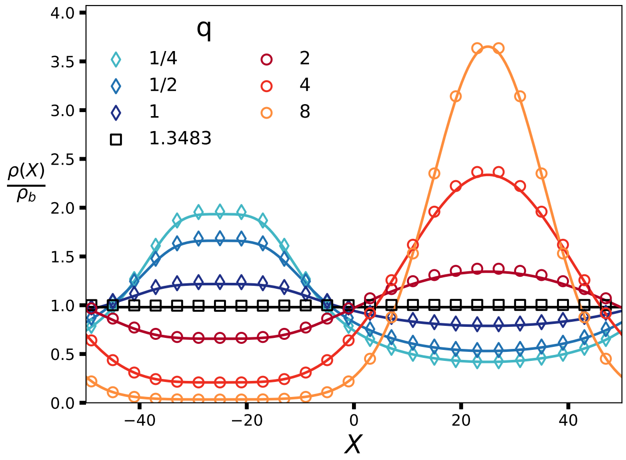


FIG. 2. Steady-state density of RTP dimers with different friction of the cargo ($q$) in one dimension with periodic boundary conditions. The theoretical prediction (lines, Eq. (138)) agrees with the numerical solution (circles) to Eqs. (118) and (119). For clarity, every other data point is shown. The swim force is $f_s(X) = 20\,(1+\sin(X2\pi/L))$ with box size $L = 100$. The spring constant is $k = 8$. Dimers with a cargo with a small friction (small $q$, blue diamonds) are anti-chemotactic and accumulate where the swim force is small (left side of the box); dimers with a cargo with a large friction (large $q$, red circles) are chemotactic and accumulate where the swim force is small (right side of the box). The cross over happens at $q \approx 1.3483$ (black squares) as predicted by Eq. (65). This behaviour is qualitatively the same as that of a dimer with a fixed bond discussed in the main text.

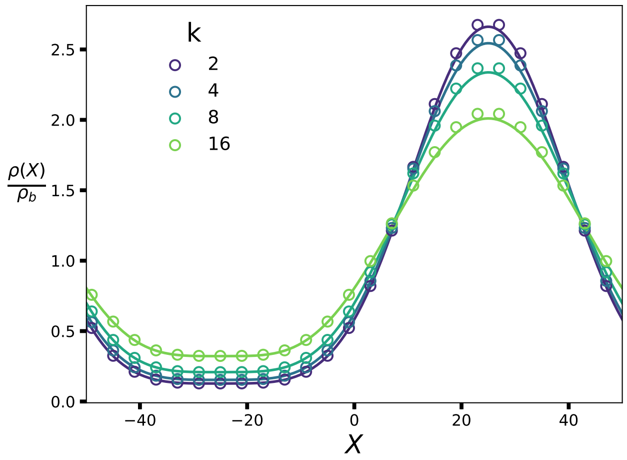


FIG. 3. Steady-state density of RTP dimers with different spring constant ($k$) in one dimension with periodic boundary conditions. The theoretical prediction (lines, Eq. (138)) agrees with the numerical solution (circles) to Eqs. (118) and (119). For clarity, every other data point is shown. The swim force is $f_s(X) = 20\,(1+\sin(X2\pi/L))$ with box size $L = 100$. The friction of the passive cargo particle is $q = 4$ times that of the active RTP particle. For this value of $q$ the dimer is chemotactic (accumulates in regions where the swim force is large). In creasing the spring constant ($k$) decreases the chemotactic behaviour because it limits the ability of the active particle to explore the space around the passive cargo particle and thus limits the dimer's ability to sense gradients in the swim force.

explore the space around the passive particle with out exerting any force, as long as the separation is smaller that the length of the 'rope' $l_0$. The behaviour of a active-passive dimer with such a potential is qualitatively similar to the cases shown before (see Fig. 4).

Because the flux (Eq. (135)) and steady-state density (Eq. (138)) are the same as the flux and steady-state density of a three-dimensional dimer (Eqs. (58) with $\epsilon$ as in Eq. (64)), one can assume that the results for the one-dimensional dimer also hold, at least qualitatively, for a two- or three-dimensional dimer. In two dimensions, an active passive dimer with a rope potential (Eq. (139)) corresponds to a active particle inside a movable ring, where the ring has the role of the passive particle. This provides a possible experimental setup to test the theory.

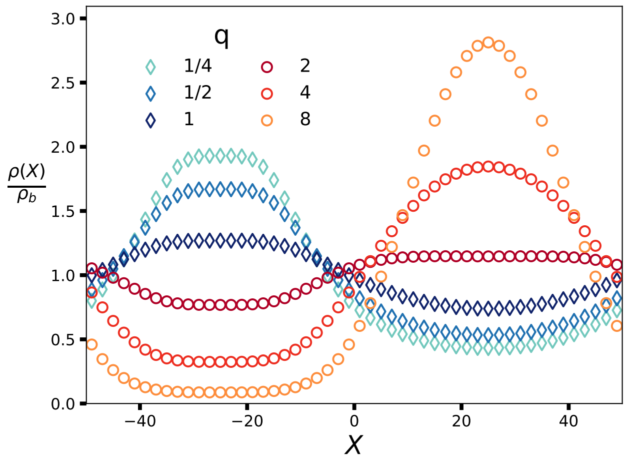


FIG. 4. Steady-state density of RTP dimers with a 'rope' potential (Eq. (139)) with $l_0 = 2$ in one dimension with periodic boundary conditions The swim force is $f_s(X) = 20\,(1+\sin(X2\pi/L))$ with box size $L = 100$. The symbols show the numerical solution to Eqs. (118) and (119).

[1] Kunihiko Kaneko. Adiabatic elimination by the eigenfunction expansion method. *Progress of Theoretical Physics*, 66(1):129–142, 1981.

[2] Mark J. Schnitzer. Theory of continuum random walks and application to chemotaxis. *Phys. Rev. E*, 48:2553–2568, Oct 1993.

[3] Michael E Cates and Julien Tailleur. When are active brownian particles and run-and-tumble particles equivalent? consequences for motility-induced phase separation. *EPL (Europhysics Letters)*, 101(2):20010, 2013.

[4] Alexandre P Solon, ME Cates, and Julien Tailleur. Active brownian particles and run-and-tumble particles: A comparative study. *The European Physical Journal Special Topics*, 224(7):1231–1262, 2015.

[5] Ayhan Duzgun and Jonathan V Selinger. Active brownian particles near straight or curved walls: Pressure and boundary layers. *Physical Review E*, 97(3):032606, 2018.

[6] Hidde Derk Vuijk, Jens-Uwe Sommer, Holger Merlitz, Joseph Michael Brader, and Abhinav Sharma. Lorentz forces induce inhomogeneity and flux in active systems. *Physical Review Research*, 2(1):013320, 2020.

[7] Clemens Bechinger, Roberto Di Leonardo, Hartmut Löwen, Charles Reichhardt, Giorgio Volpe, and Giovanni Volpe. Active particles in complex and crowded environments. *Rev. Mod. Phys.*, 88:045006, 2016.

[8] Hannes Risken. Fokker-planck equation. In *The Fokker-Planck Equation*, pages 63–95. Springer, 1996.

[9] Philip McCord Morse, Herman Feshbach, et al. *Methods of Theoretical Physics*, volume 1. McGraw-Hill New York, 1953.

[10] Michael te Vrugt and Raphael Wittkowski. Relations between angular and cartesian orientational expansions. *AIP Advances*, 10(3):035106, 2020.

[11] Pierre-Gilles De Gennes and Jacques Prost. *The physics of liquid crystals*, volume 83. Oxford university press, 1993.

[12] Aparna Baskaran and M Cristina Marchetti. Hydrodynamics of self-propelled hard rods. *Physical Review E*, 77(1):011920, 2008.

[13] A. Sharma and J.M. Brader. Brownian systems with spatially inhomogeneous activity. *Phys. Rev. E*, 96:032604, 2017.

[14] Max Born and Robert Oppenheimer. Zur quantentheorie der molekeln. *Annalen der physik*, 389(20):457–484, 1927.

[15] J. Tailleur and M. E. Cates. Sedimentation, trapping, and rectification of dilute bacteria. *EPL (Europhysics Letters)*, 86(6):60002, 2009.

[16] AY Grosberg and J-F Joanny. Nonequilibrium statistical mechanics of mixtures of particles in contact with different thermostats. *Physical Review E*, 92(3):032118, 2015.

[17] Simon N Weber, Christoph A Weber, and Erwin Frey. Binary mixtures of particles with different diffusivities demix. *Physical review letters*, 116(5):058301, 2016.

[18] Efe Ilker and Jean-François Joanny. Phase separation and nucleation in mixtures of particles with different temperatures. *Physical Review Research*, 2(2):023200, 2020.

[19] Michael Wang and Alexander Y Grosberg. Three-body problem for langevin dynamics with different temperatures. *Physical Review E*, 101(3):032131, 2020.

[20] Demian Levis and Ludovic Berthier. From single-particle to collective effective temperatures in an active fluid of self-propelled particles. *EPL (Europhysics Letters)*, 111(6):60006, 2015.

[21] Grzegorz Szamel. Self-propelled particle in an external potential: Existence of an effective temperature. *Physical Review E*, 90(1):012111, 2014.

[22] NG Van Kampen. Diffusion in inhomogeneous media. *Zeitschrift für Physik B Condensed Matter*, 68(2-3):135–138, 1987.

[23] J Tailleur and ME Cates. Statistical mechanics of interacting run-and-tumble bacteria. *Physical review letters*, 100(21):218103, 2008.
